# Supplementary material for: Prediction of Workplace Injuries
Source: arXiv:1906.03080 source file (2019-06-05)
Supplement: Supplementary file 1 [file supp.pdf]

## Supplementary Material

### 1. Transfer Learning

Given a loss function  $\mathcal{L}(\cdot)$  and a set of target training samples  $\{(x_i, y_i) | i \in \{1, 2, \dots, N_T\}\}$ , the goal of supervised learning is to find model  $\mathcal{A}^*$  that minimizes the expected error, *i.e.*,  $\mathcal{A}^* = \arg \min_{\mathcal{A} \in \mathbb{A}} \mathbb{E}_{x \sim P_T} [\mathcal{L}(\mathcal{A}(x), y)]$ . Here  $x$  is an arbitrary sample and  $P_T$  is the probability distribution of target samples. We follow the idea of importance sampling (Liu, 2008; Asgarian et al., 2018) to transfer the knowledge from source domain ( $S$ ) to target domain ( $T$ ). Assuming an infinite number of training samples, we can express the expected error based on the samples from target and source domains as follows (Haase et al., 2014).

$$\begin{aligned} \mathbb{E}_{x \sim P_T} [\underbrace{\mathcal{L}(\mathcal{A}(x), y)}_{\epsilon(x)}] &= \int \epsilon(x) P_T(x) dx \\ &= \int \epsilon(x) \underbrace{\left[ \alpha + (1 - \alpha) \frac{P_S(x)}{P_S(x)} \right]}_{=1} P_T(x) dx \\ &= \alpha \mathbb{E}_{x \sim P_T} [\epsilon(x)] + (1 - \alpha) \mathbb{E}_{x \sim P_S} \left[ \underbrace{\epsilon(x) \frac{P_T(x)}{P_S(x)}}_{w_x} \right] \end{aligned} \quad (1)$$

Here  $\epsilon(x)$  shows the error for each sample and  $\alpha$  is a hyper-parameter that controls the overall relative importance between source and target samples. Source sample weights  $\{w_{x_j} = \frac{P_T(x_j)}{P_S(x_j)} \mid j \in \{1, \dots, N_S\}\}$  have a major role in instance-based transfer learning methods, as they control the individual effect of source samples. Considering the case where a finite number of source ( $N_S$ ) and target ( $N_T$ ) training samples are available, we can replace the expected values and other terms in Equation 1 with their respective counterparts.

$$\Theta^* = \arg \min_{\Theta} \left( \frac{\alpha}{N_T} \sum_{i=1}^{N_T} \epsilon(x_i, \Theta) + \frac{1 - \alpha}{N_S} \sum_{j=1}^{N_S} \epsilon(x_j, \Theta) w_{x_j} \right) \quad (2)$$

Models  $\mathcal{A}_S$ ,  $\mathcal{A}_T$ , and  $\mathcal{A}_{S \cup T}$  trained respectively on source, target and the union of source and target, serve as minimum baselines that a transfer learning method must outperform. Our fourth baseline model is an instance-weighted model ( $\mathcal{A}_1$ ) with all the weights set to 1 (*i.e.*,  $\mathbf{W}_S = \mathbf{1}$ ). This is similar to  $\mathcal{A}_{S \cup T}$ , except in this model we use  $\alpha$  to determine the relative overall importance between source and target samples.

Our last baseline model ( $\mathcal{A}_G$ ), assumes Gaussian distributions for target and source samples, which leads to  $w_{x_j} = \frac{P_T(x_j)}{P_S(x_j)} = \frac{N(x_j; \mu_T, \Sigma_T)}{N(x_j; \mu_S, \Sigma_S)}$ . Here  $\mu_T$  and  $\mu_S$  show the mean and  $\Sigma_T$  and  $\Sigma_S$  show the covariance matrices for target and source distributions respectively. We call this model with  $\mathcal{A}_G$ .

**Hybrid Weights:** Previous methods evaluate the source sample weights solely based on their similarity to the target domain. We argue that it is also important to measure the relevance of source samples to the target task. Hence, we define weights  $w_x = w_{domain_x} + w_{task_x}$ , where  $w_{domain_x}$  measures the similarity of an arbitrary source sample  $x$  to the target domain, while  $w_{task_x}$  measures the importance of sample  $x$  in the target task.

For evaluating  $w_{domain_x}$ , unlike the previous methods that employ generative approaches to estimate  $P_T$  and  $P_S$ , we directly approximate weights  $w_{domain_x} = \frac{P_T(x)}{P_S(x)}$  with a discriminative classifier. More specifically, using  $\{(x, l_x) \mid x \in S \cup T, \text{ and } l_x = 1 \text{ if } x \in S, l_x = 0 \text{ otherwise}\}$ , we train a binary classifier (e.g., logistic regression (LR)) to differentiate source and target samples. Next, we use the learned weights of this classifier ( $w_{lr}$  and  $c_{lr}$ ) to estimate source sample weights  $w_{domain_x} = \frac{P_T(x)}{P_S(x)} \approx \frac{1}{\exp(x^T w_{lr} + c_{lr})}$ .

To compute  $w_{task_x}$ , we train an instance of our predictive model (XGBoost) using all samples from source and target with their corresponding injury labels. We then define  $w_{task_x}$  to be the uncertainty of this model about sample  $x$ . We define the uncertainty of a model about sample  $x$  to be the distance of  $x$  to the decision boundary. Note that this value could be negative (thus subtracting from  $w_x$ ) when the decision is incorrect, or positive (thus adding to  $w_x$ ) when the decision is correct. We denote this model as  $\mathcal{A}_{HW}$ .

### 2. Additional Results

Table 1 shows the performance of various methods on positive (injury) class and negative class. As it can be seen, the performance of all methods is very high on negative class and relatively very low on positive class, which could be explained by the imbalance issues in the dataset. The trend is that almost all instance-based methods perform better compared to the baseline models  $\mathcal{A}_T$ ,  $\mathcal{A}_S$ , and  $\mathcal{A}_{S \cup T}$ , highlighting the effect of transfer learning. Among instance-based transfer learning methods, our model  $\mathcal{A}_{HW}$  has the best performance in terms of  $F_1$ -score and AUCPR while having a high  $F_1$ -score on the negative class.

Figure 1 shows the feature importance scores obtained with target-only model ( $\mathcal{A}_T$ ) and our model ( $\mathcal{A}_{HW}$ ). We can see that model  $\mathcal{A}_T$  has a very low importance score for 25 features from the 38 engineered features and mainly considers 13 features. Among these 25 features, we can see features like the number of illnesses (illness), if employee are technician or laborers (jobtype.technician and jobtype.laborer), if employees are working full-time (workstatus.full-time). However, our model  $\mathcal{A}_{HW}$  utilizes 23 features which includes  $\mathcal{A}_T$ 's 13 features plus 10 more features including the number of illnesses, if employee are technician or laborers, and if they are working full-time.

| Methods             | Positive Class |        |                       |        | Negative Class |        |                       |
|---------------------|----------------|--------|-----------------------|--------|----------------|--------|-----------------------|
|                     | Precision      | Recall | F <sub>1</sub> -score | AUCPR  | Precision      | Recall | F <sub>1</sub> -score |
| $\mathcal{A}_T$     | 0.07           | 0.06   | 0.06                  | 0.0375 | 0.98           | 0.99   | 0.99                  |
| $\mathcal{A}_S$     | 0.04           | 0.18   | 0.07                  | 0.0405 | 0.99           | 0.93   | 0.96                  |
| $\mathcal{A}_{SUT}$ | 0.13           | 0.06   | 0.08                  | 0.0478 | 0.98           | 0.99   | 0.99                  |
| $\mathcal{A}_I$     | 0.06           | 0.12   | 0.08                  | 0.0456 | 0.99           | 0.97   | 0.98                  |
| $\mathcal{A}_G$     | 0.07           | 0.16   | 0.10                  | 0.0532 | 0.99           | 0.97   | 0.98                  |
| $\mathcal{A}_{HW}$  | 0.11           | 0.12   | 0.12                  | 0.0542 | 0.99           | 0.98   | 0.98                  |

Table 1. Per class performance of different methods on Company-1’s data.

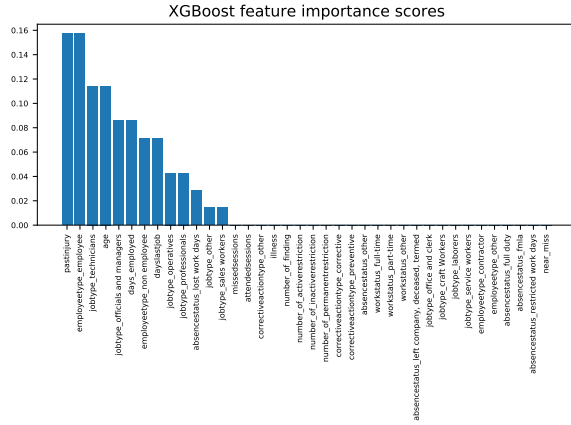

(a) Features importance scores for model  $\mathcal{A}_T$ .

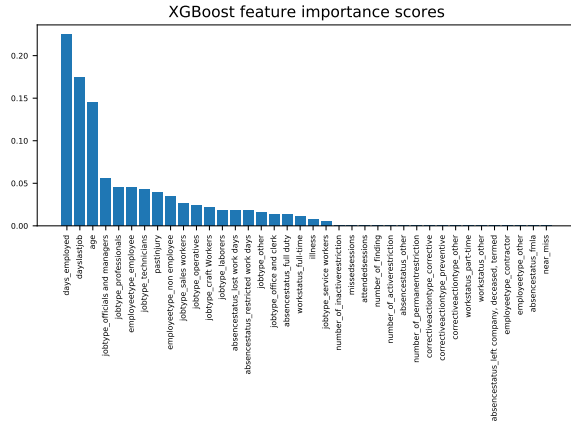

(b) Features importance scores for model  $\mathcal{A}_{HW}$ .

Figure 1. Illustration of feature importance scores obtained with target-only model ( $\mathcal{A}_T$ ) and our hybrid model ( $\mathcal{A}_{HW}$ ). Company names are masked for confidentiality reasons.

## References

- Asgarian, A., Sobhani, P., Zhang, J. C., Mihailescu, M., Sibilia, A., Ashraf, A. B., and Taati, B. A hybrid instance-based transfer learning method. *arXiv:1812.01063*, 2018.
- Haase, D., Rodner, E., and Denzler, J. Instance-weighted transfer learning of active appearance models. In *2014 IEEE CVPR*, 2014.
- Liu, J. S. *Monte Carlo strategies in scientific computing*. Springer Science & Business Media, 2008.
